# Supplementary material for: Ground and Excited State First-Order Properties in Many-Body Expanded Full Configuration Interaction Theory
Source: arXiv:2008.03610 ancillary file (2020-10-16)
Supplement: Supplementary file 1 [file si.pdf]

# Supporting Information: Ground and Excited State First-Order Properties in Many-Body Expanded Full Configuration Interaction Theory

Janus J. Eriksen*,† and Jürgen Gauss*,‡

†*School of Chemistry, University of Bristol, Cantock's Close, Bristol BS8 1TS, United Kingdom*

‡*Department Chemie, Johannes Gutenberg-Universität Mainz, Duesbergweg 10-14, 55128 Mainz, Germany*

E-mail: janus.eriksen@bristol.ac.uk; gauss@uni-mainz.de

# 1 Tabulated Results

**Table S1:** Raw data (in au) behind Figure 1 of the main study.

| Basis Set | Method | Property | | |
|---|---|---|---|---|
| | | $E^{0n}$ | $\mu^n$ | $t^{0n}$ |
| 1st Excited State ($^1\Sigma^+$) | | | | |
| aug-cc-pVDZ | MBE-FCI | 0.130442 | −2.020053 | −0.965058 |
| | *i*-FCIQMC | 0.130434 | −2.01947 | −0.965189 |
| aug-cc-pVTZ | MBE-FCI | 0.132487 | −2.025952 | −0.935688 |
| | *i*-FCIQMC | 0.132458 | −2.02541 | −0.93538 |
| aug-cc-pVQZ | MBE-FCI | 0.132999 | −2.021608 | −0.926786 |
| | *i*-FCIQMC | 0.132943 | −2.0188 | −0.92658 |
| 2nd Excited State ($^1\Sigma^+$) | | | | |
| aug-cc-pVDZ | MBE-FCI | 0.214984 | 3.330613 | 0.375607 |
| | *i*-FCIQMC | 0.214980 | 3.3543 | 0.37471 |
| aug-cc-pVTZ | MBE-FCI | 0.216731 | 3.778210 | 0.413522 |
| | *i*-FCIQMC | 0.216705 | 3.794 | 0.41146 |
| aug-cc-pVQZ | MBE-FCI | 0.217656 | 3.672453 | 0.401169 |
| | *i*-FCIQMC | 0.217616 | 3.696 | 0.3984 |

**Table S2:** Raw data (in au) behind Figure 2 of the main study.

| Basis Set | Method | Property $E^n$ | Property $\mu^n$ |
|---|---|---|---|
| Ground State ($^1\Sigma^+$) | | | |
| aug-cc-pVDZ | MBE-FCI | $-274.653412$ | 2.387267 |
| | *i*-FCIQMC | $-274.654$ | 2.382 |
| 1st Excited State ($^1\Sigma^+$) | | | |
| aug-cc-pVDZ | MBE-FCI | $-274.564609$ | 2.253221 |
| | *i*-FCIQMC | $-274.564$ | 2.289 |
| 2nd Excited State ($^1\Sigma^+$) | | | |
| aug-cc-pVDZ | MBE-FCI | $-274.516964$ | 1.144318 |
| | *i*-FCIQMC | $-274.517$ | 1.154 |

## 2 LiH: Ground State ($^1\Sigma^+$)

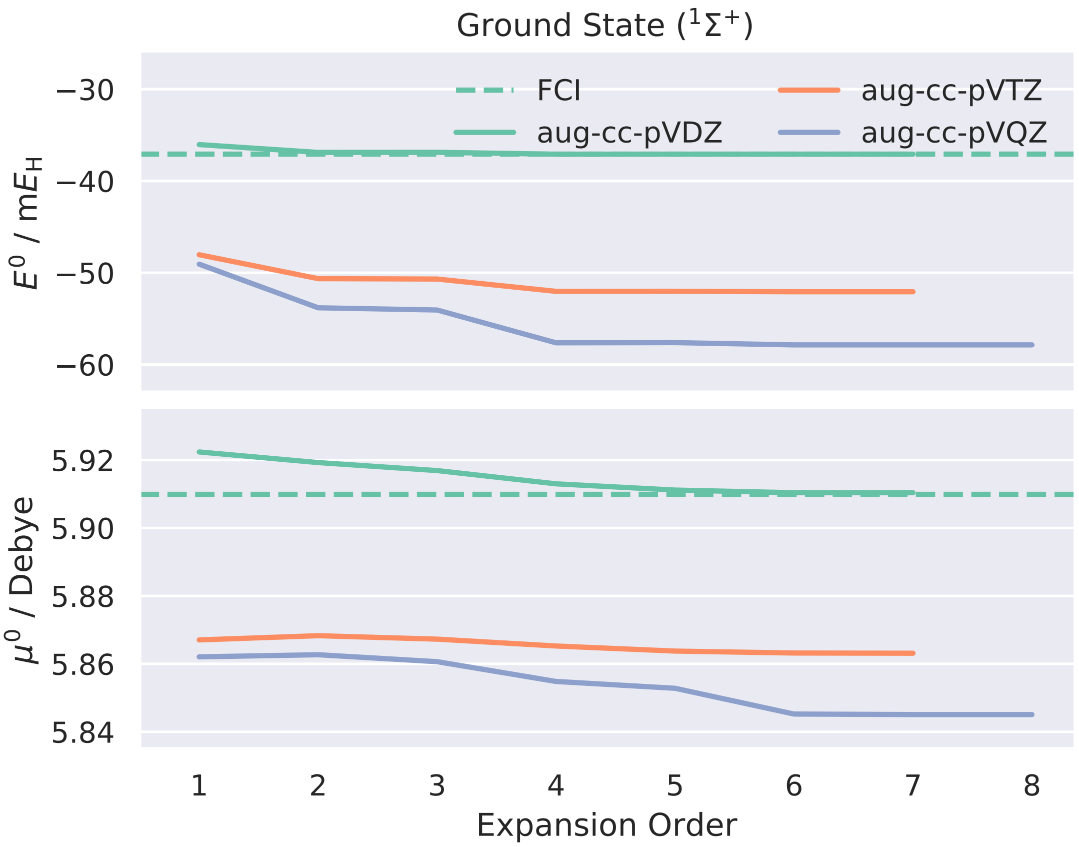


**Figure S1:** Ground state ($^1\Sigma^+$ symmetry) correlation energies ($E^0$, upper panel) and dipole moments ($\mu^0$, lower panel) for LiH in the aug-cc-pV$XZ$ basis sets. Solid and dashed lines denote MBE-FCI and FCI results, respectively.

# 3 LiH: $\pi$-pruning

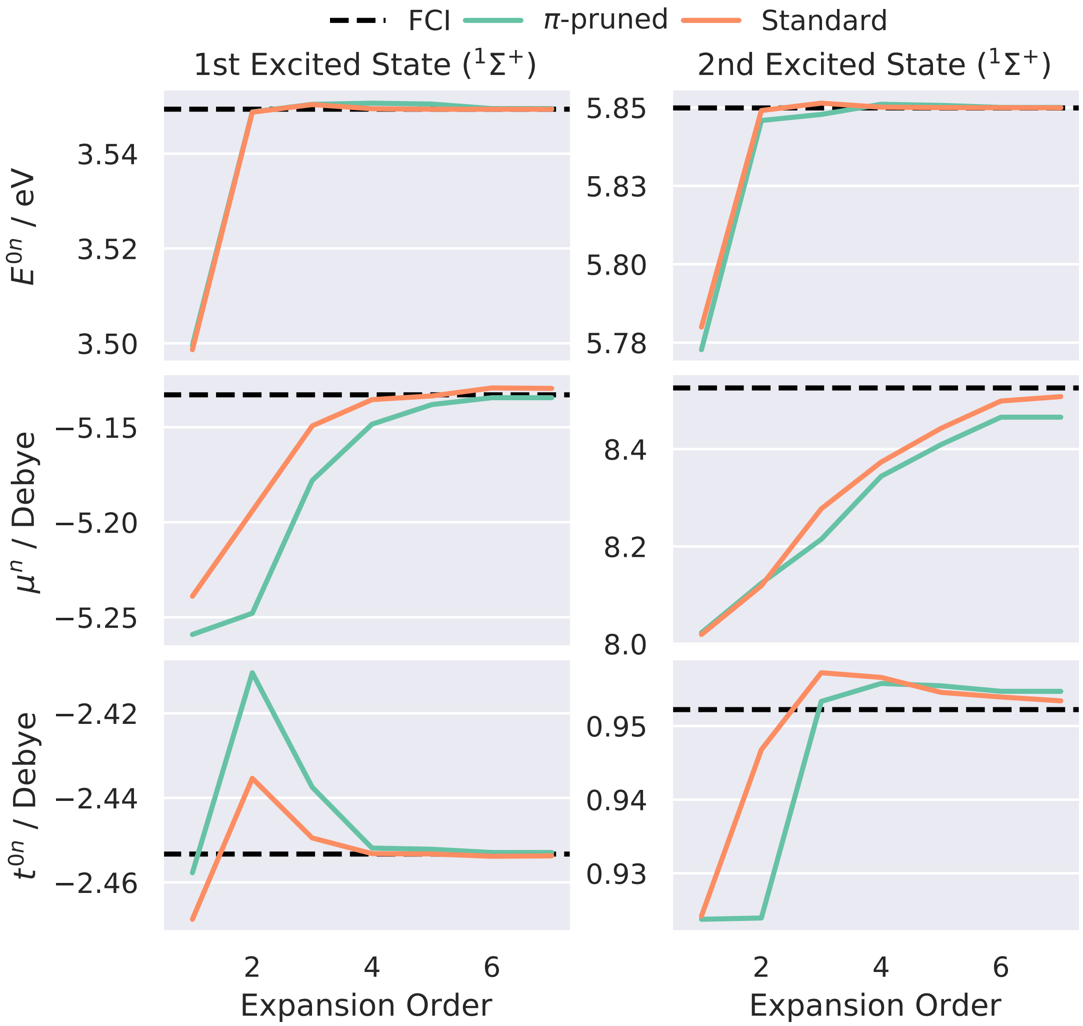


**Figure S2:** Excitation energies ($E^{0n}$, upper panels), dipole moments ($\mu^n$, center panels), and transition dipole moments ($t^{0n}$, lower panels) for the first two excited states ($^1\Sigma^+$ symmetry) of LiH in the aug-cc-pVDZ basis sets. Results are presented with $\pi$-pruning or without (standard).

# 4 LiH: Tighter Screening Thresholds

In the 'normal' screening protocol, which is the one used throughout the main study unless specified otherwise, no screening takes place at order $k \leq 5$. At order $k = 6$, the 50 % of the expansion space which contributes the least is screened away, 75 % at order $k = 7$, and 87.5 % at order $k = 8$. In the 'tight' screening protocol, no screening takes place at order $k \leq 7$ followed by a screening of 20 % at all subsequent orders.

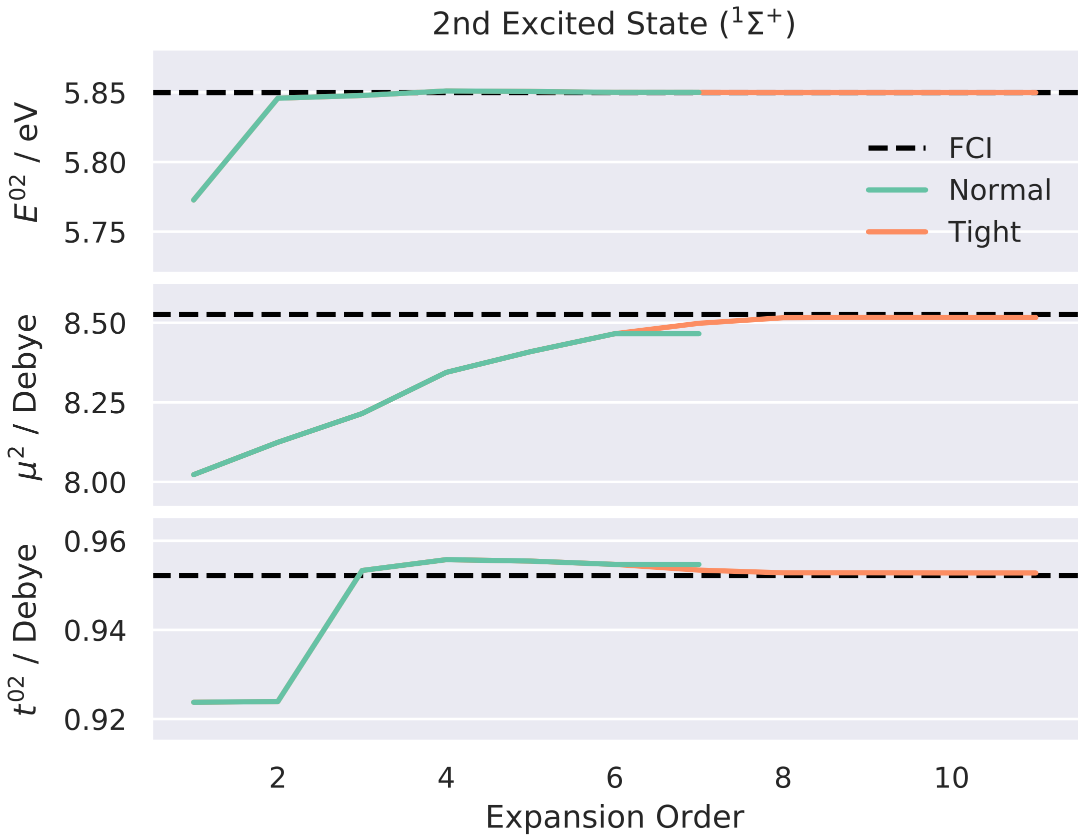


**Figure S3:** Excitation energies ($E^{02}$, upper panels), dipole moments ($\mu^2$, center panels), and transition dipole moments ($t^{02}$, lower panels) for the 2nd excited state ($^1\Sigma^+$ symmetry) of LiH in the aug-cc-pVDZ basis sets. Results are presented using $\pi$-pruning and normal as well as tight screening thresholds.
